# Supplementary material for: A roadmap for the computation of persistent homology
Source: arXiv:1506.08903 ancillary file (2017-09-12)
Supplement: Supplementary file 1 [file Additional_Computations.pdf]

## ADDITIONAL COMPUTATIONS

**1. Introduction.** We report additional computations that we perform with the libraries that we study. See the main paper for a description of the data sets and details on how we perform the computations.

**2. Vietoris–Rips complex.** In this section, we report additional results for the computation of PH with the VR complex, as explained in Section 7 of the main manuscript. In Tables 1–4, we give results for the computations on a cluster; in Table 5, we give results for the computations on a shared-memory system. For the data set **Vicsek**, we computed PH for six different point clouds, as we also explain in the main paper. We report results only for one of these points clouds, because the results of the computations — in terms of wall-time seconds and memory used — were all similar. The point cloud for which we report the results has the following parameters (see the main manuscript for a discussion of these parameters):  $N = 300$ ,  $l = 5$ ,  $\theta_0 = 1$ ,  $v_0 = 0.03$ ,  $\eta = 0.1$ , and  $T = 600$ . Of the 600 different points clouds (one for each time step  $t$ ), we choose the one that corresponds to time step  $t = 300$ .

TABLE 1

*Computations of PH with VR complex for the data set **drag 1**. The size of the complex is  $1.7 \times 10^8$ , and the dimension is 2. We run DIPHA on one node and 16 cores.*

|               | Wall-time seconds | CPU seconds | Memory in GB |
|---------------|-------------------|-------------|--------------|
| JAVAPLEX (st) | -                 | -           | > 64         |
| DIONYSUS (st) | -                 | -           | -            |
| DIPHA (st)    | 7356              | 117417      | 2.4          |
| PERSEUS       | -                 | -           | -            |
| DIONYSUS (d)  | 4360              | 4362        | 16.8         |
| DIPHA (d)     | 75                | 1176        | 1.8          |
| GUDHI         | 1524              | 1517        | 7.9          |
| RIPSER        | 2                 | 1           | 0.04         |

TABLE 2

*Computations of PH with VR complex for the data set **house**. The size of the complex is  $1.6 \times 10^9$ , and the dimension is 3. We run DIPHA (d) on three nodes of 16 cores, and DIPHA (st) on four nodes of 16 cores.*

|               | Wall-time seconds | CPU seconds | Memory in GB |
|---------------|-------------------|-------------|--------------|
| JAVAPLEX (st) | -                 | -           | > 64         |
| DIPHA (st)    | 53686             | 243587      | 5.3          |
| PERSEUS       | -                 | -           | -            |
| DIONYSUS (d)  | -                 | -           | -            |
| DIPHA (d)     | 1450              | 22981       | 7.1          |
| GUDHI         | 46377             | 25925       | 64.6         |
| RIPSER        | 11                | 11          | 0.8          |

**3. Image data set.** In this section, we report timings and memory usage for the computation of PH with cubical complexes with the libraries DIPHA, PERSEUS, and GUDHI for the data set **vertebra**. For this data set, the standard implementation in DIPHA performs better in terms of wall time, CPU seconds, and memory usage than the dual implementation. This does not necessarily contradict the fact that the dual implementation gives a heuristic speed-up with respect to the standard imple-

TABLE 3

Computations of PH with VR complex for the data set *senate*. The size of the complex is  $4.6 \times 10^6$ , and the dimension is 3. We run DIPHA on two nodes and 16 cores.

|               | Wall-time seconds | CPU seconds | Memory in GB |
|---------------|-------------------|-------------|--------------|
| JAVAPLEX (st) | 222               | 571         | < 5          |
| DIPHA (st)    | 5                 | 58          | 0.1          |
| PERSEUS       | 457               | 457         | 4.9          |
| DIONYSUS (d)  | 183               | 183         | 0.5          |
| DIPHA (d)     | 5                 | 34          | 0.1          |
| GUDHI         | 51                | 51          | 0.2          |
| RIPSER        | 1                 | 1           | 0.01         |

TABLE 4

Computations of PH with VR complex for the data set *netw-sc*. The size of the complex is  $8.5 \times 10^8$ , and the dimension is 3. We run DIPHA on two nodes of 16 cores.

|               | Wall-time seconds | CPU seconds | Memory in GB |
|---------------|-------------------|-------------|--------------|
| JAVAPLEX (st) | -                 | -           | > 64         |
| DIPHA (st)    | 16004             | 202755      | 5.6          |
| PERSEUS       | -                 | -           | -            |
| DIONYSUS (d)  | -                 | -           | -            |
| DIPHA (d)     | 618               | 9842        | 5.8          |
| GUDHI         | 13483             | 13465       | 40.6         |
| RIPSER        | 9                 | 9           | 0.5          |

TABLE 5

Computations on the shared-memory system.

| Data set        | <b>H3N2</b>       | <b>Vicsek</b>     | <b>drag 1</b>     | <b>fract 1</b>    |
|-----------------|-------------------|-------------------|-------------------|-------------------|
| Size of complex | $3.4 \times 10^9$ | $3.3 \times 10^8$ | $1.7 \times 10^8$ | $2.8 \times 10^9$ |
| Max. dim.       | 2                 | 3                 | 2                 | 3                 |
| JAVAPLEX (st)   | -                 | 26257             | 19054             | -                 |
| PERSEUS         | -                 | -                 | -                 | -                 |
| DIONYSUS (d)    | -                 | 4637              | 2889              | 593528            |
| DIPHA (d)       | 14362             | 369               | 1775              | 3920              |
| GUDHI           | 3377              | 433               | 144               | 4154              |
| RIPSER          | 24                | 3                 | 2                 | 14                |

(a) Computations on the shared-memory system: wall-time seconds

| Data set        | <b>H3N2</b>       | <b>Vicsek</b>     | <b>drag 1</b>     | <b>fract 1</b>    |
|-----------------|-------------------|-------------------|-------------------|-------------------|
| Size of complex | $3.4 \times 10^9$ | $3.3 \times 10^8$ | $1.7 \times 10^8$ | $2.8 \times 10^9$ |
| Max. dim.       | 2                 | 3                 | 2                 | 3                 |
| JAVAPLEX (st)   | > 700             | < 600             | < 600             | > 700             |
| PERSEUS         | -                 | -                 | -                 | -                 |
| DIONYSUS (d)    | -                 | 33.5              | 16.8              | 269               |
| DIPHA (d)       | 276.1             | 32.5              | 13.8              | 276.1             |
| GUDHI           | 158.2             | 15.9              | 7.9               | 134.5             |
| RIPSER          | 0.2               | 0.3               | 0.04              | 1.2               |

(b) Computations on the shared-memory system: memory in GB

mentation, because it is well-known that the dual implementation gives a speed-up when one computes PH with the VR complex but not in general.

TABLE 6

Computations of PH with cubical complexes for the data set *vertebra* on the shared-memory system. The complex, as constructed by DIPHA and GUDHI, has  $1.1 \times 10^9$  cells, and its dimension is 3. Note that PERSEUS implements a less efficient way for building filtered cubical complexes from grey-scale images, and the resulting complex has more cells than the one constructed by DIPHA and GUDHI.

|                   | DIPHA (d) | DIPHA (st) | PERSEUS | GUDHI (d) |
|-------------------|-----------|------------|---------|-----------|
| Wall-time seconds | 2115      | 1793       | 19604   | 3668      |
| Memory in GB      | 82.1      | 80.9       | 628.8   | 59.8      |

**4. Additional functionalities.** In this section, we report timings and memory usage for the computation of PH with the alpha ( $\alpha$ ), Čech ( $\check{C}$ ), weak witness complex (W), and parametrized witness complex for  $\nu = 2$  ( $W_2$ ) (see the main text for a description of these complexes). For the witness complexes we choose the landmark points uniformly at random. We use the two data sets consisting of point clouds in  $\mathbb{R}^3$  (i.e., the data sets **Klein** and **Vicsek**). Additionally, note that the newest version of GUDHI (Version 1.3.1) implements the computation of witness complexes, but it does not implement the computation of filtered witness complexes.

TABLE 7

Computations of alpha and Čech complexes on the shared-memory system.

|                   | DIONYSUS $\alpha$ | DIONYSUS $\check{C}$ | GUDHI $\alpha$    |
|-------------------|-------------------|----------------------|-------------------|
| Size of complex   | $9.2 \times 10^3$ | -                    | $9.2 \times 10^3$ |
| Wall-time seconds | 1                 | -                    | 2                 |
| Memory in GB      | 0.008             | -                    | 0.006             |

(a) Time and memory usage for the data set **Klein**.

|                   | DIONYSUS $\alpha$ | DIONYSUS $\check{C}$ | GUDHI $\alpha$    |
|-------------------|-------------------|----------------------|-------------------|
| Size of complex   | $7.7 \times 10^3$ | -                    | $7.7 \times 10^3$ |
| Wall-time seconds | 1                 | -                    | 2                 |
| Memory in GB      | 0.007             | -                    | 0.006             |

(b) Time and memory usage for the data set **Vicsek**. For the witness complexes we choose 100 landmark points uniformly at random.

TABLE 8

*Computations of PH with the witness complex on the shared-memory system.*

|                   | JAVAPLEX W        | JAVAPLEX W <sub>2</sub> |
|-------------------|-------------------|-------------------------|
| Size of complex   | $6.8 \times 10^5$ | $2.8 \times 10^6$       |
| Wall-time seconds | 32                | 328                     |
| Memory in GB      | < 2               | < 5                     |

(a) Time and memory usage for the data set **Klein**. We choose 100 landmark points uniformly at random.

|                   | JAVAPLEX W      | JAVAPLEX W <sub>2</sub> |
|-------------------|-----------------|-------------------------|
| Size of complex   | $1 \times 10^6$ | $4.1 \times 10^6$       |
| Wall-time seconds | 50              | 84                      |
| Memory in GB      | < 3             | < 5                     |

(b) Time and memory usage for the data set **Vicsek**. For the witness complexes, we choose 100 landmark points uniformly at random.
